# Supplementary material for: Regularizing Generative Adversarial Networks under Limited Data
Source: arXiv:2104.03310 source file (2021-04-07)
Supplement: Supplementary file 1 [file ffhq.tex]

\begin{table*}[t]
    \caption{\textbf{Comparisons with other GANs on the \FFHQ dataset.} We report the average FID scores ($\downarrow$) of three evaluation runs. The best performance is in \textbf{bold} and the second best is \underline{underscored}.}
    \vspace{\tabcapmargin}
    \label{tab:supp_ffhq}
    \centering
    \footnotesize
    \begin{tabular}{l|ccccc|ccc} 
	    \toprule
		Method & PA-GAN~\cite{} & WGAN-GP~\cite{wgangp} & bCR~\cite{zhao2020bcr} & \thead{Auxiliary\\rotation~\cite{}} & \thead{Spectral\\norm~\cite{}} & StyleGAN2~\cite{stylegan2} & +ADA~\cite{ada} & \thead{+ADA + $R_\mathrm{LC}$\\(\textbf{Ours})} \\
	    \midrule
	    Full & $3.78${\mytiny$\pm.06$} & $6.54${\mytiny$\pm.37$} & $3.45${\mytiny$\pm.19$} & $4.16${\mytiny$\pm.05$} & $4.60${\mytiny$\pm.19$} & $3.66${\mytiny$\pm.10$} & $3.82${\mytiny$\pm.01$} & $\best{3.49}${\mytiny$\pm0.04$} \\
	    2$k$ & $56.49${\mytiny$\pm7.3$} & $6.54${\mytiny$\pm.37$} & $3.45${\mytiny$\pm.19$} & $4.16${\mytiny$\pm.05$} & $4.60${\mytiny$\pm.19$} & $3.66${\mytiny$\pm.10$} & $3.82${\mytiny$\pm.01$} & $\best{3.49}${\mytiny$\pm0.04$} \\
		\bottomrule
    \end{tabular}
    \vspace{\tabbotmargin}
    \vspace{-1mm}
\end{table*}
